# Supplementary material for: Active Inference and Human--Computer Interaction
Source: arXiv:2412.14741 source file (2024-12-19)
Supplement: Supplementary file 1 [file appendix.tex]

\section{Holding ground}

\subsection{AI and algorithmic automation: } 
 Algorithmic support from artificial intelligence will be a common element of future interaction. New technologies such as deep networks and large language models offer powerful ways for systems to interpret signals such as images, sound and text. This complex algorithmic manipulation of observations or states can add value by extending our perception, cognition or actuation capabilities, but in the end, it needs to be controlled by the user for successful interaction -- human users will need to be able to reason about and control the level of autonomy available when interacting with a system. So the question remains: how can we use this in design in a principled manner? Active inference provides a framework for incorporating algorithmic processing components in the same way as a rich sensor or actuator (or more generally, tools, which would group subsets of action and sensing nodes), and allows the agent to adjust its uncertainty in managing the complexity involved.

%\TODO{There is another point here; ML algorithms clearly extend perception and actuation of artificial agents, but largely don't do anything to improve interaction itself}

\section{Removed lamp content}
%Additional capabilities could be added by extending the lamp's sensorium. An orientation sensor could be added so that the lamp can perceive how it is posed. This can form part of its predictive model, so that it can (for example) anticipate and brighten as it is brought to a surface for close work, without explicit user adjustment. 

%Extending the lamp's prediction to horizon to long term, we can conceive of it in the original framing of active inference as a (synthetic) organism with a goal to survive by resisting entropy. Minimising surprise means minimising the risk of being switched off forever. This motivates the lamp to temper its enthusiasm for engaging the user to avoid frustration and anger. 
%\TODO{sharing of state over many lamp generations}

%%%%%%%

\subsubsection*{What is AIF not good for?}

Most compelling immediate applications are in interaction with novel rich sensors and sharing control with semi-autonomous tools?

\section{Theories in Human--Computer Interaction}

Antti book: ``how can people with different goals and capabilities, and in different contexts, be able to use computing productively, enjoyably, and safely?''

\subsection{What are HCI theories?}

Theories in HCI paper \cite{lamas2024hci} \cite{oulasvirta2022counterfactual}

Over three decades ago \cite{winograd1990can} asked `What is interaction?'. A recent paper by \citet{hornbaek2017interaction}
 discussed the competing concepts of interaction in more detail  and subsequently \cite{hornbaek2019we} reviewed the literature at ACM SIG CHI on `interaction'. From this perspective an active inference approach would fundamentally correspond to elements of their classifications of {\it `Interaction as Control'} and {\it`Interaction as Information transmission'}, but because of the consequences of the predictive agent-focused approach, it would also incorporate {\it Interaction as tool use, Interaction as Optimal Behaviour, and Interaction as Embodied Action}.

 \cite{janlert2017meaning}.

{\it ``Interaction.. is something fluid, a dynamic process played out in time..'', ``The interface appears more designable than the interaction''}, \cite{janlert2017things}. Can we develop models which represent, and hence quantify, the nature of the dynamic evolution of interaction between agents, independent of interface specifics?

Interaction fields \cite{janlert2022emergence}
\cite{janlert2015faceless}

Interface bottleneck \cite{janlert2017things},p8.

%\cite{sheridan2016modeling,She02}

%Bunge \cite{bunge2017causality} sees interaction as {\it reciprocal causation}, as in gravity, and proposed approaches based on as a special type of causal relationship applied in scientific explanation: {\it Mutual determination}, rather than a traditional {\it causal determination} approach. The point of mutual determination that what happens in interaction is mutually determined by the human and the computer. Interaction cannot be attributed solely to the human or the computer alone: the two must be considered together. %HorKriOul24 book

%    As Mackay says,  it may be better to focus on {\it interdependence} rather than traditional {\it causality} when examining closed-loop interactions in complex multi-level systems \cite{mackay1991behind}, p63. This means that some concepts can only be quantitatively measured as part of a model of the whole interaction loop.\\

`Teleological determination' is about the human's intentions defining a norm or goal for interaction.  AIF does this via the priors.

\subsubsection{Explanatory power}
A theory of HCI should have explanatory power, it should have empirical accuracy and broad scope. It should shed light on latent or unobservable factors. Which factors can AIF shed light on? Can it explain how some surprising and important phenomena in HCI emerge? 
% from HorKriOul24 book
\subsubsection{Predictive power}
Our theories should also enable predictions.

\subsubsection{Evaluation power}
Our theoretical frameworks should also help us evaluate interaction.

\subsubsection{Guiding measurement}
\subsubsection{Informing design}
HCI is concerned with design and engineering, so we need our theory to help us reason about design.

\subsection{Requirements}

\subsubsection{HCI}
On tasks:
\begin{itemize}
    \item Complex task structures require several actions to be taken successfully to achieve goals. This is challenging for short-term control approaches.
\end{itemize}

%On interaction:
%\begin{itemize}
%    \item Interaction is fundamentally a closed-loop process, so components in the interaction loop cannot be meaningfully analysed independently. It is challenging to establish causality between inputs and outputs, or even to determine what should be called an `input' and what an `output'. 

%    LINK TO BUNGE DISCUSSION
%\end{itemize}

%Challenges relating to design:
%\begin{itemize}
%\item Design is hard and involves many trade-offs. Forcing designers to pin down everything in advance, in ignorance of the specific user, context and task is challenging. Being able to leave some of the adaptation to deployment, such that users and interfaces can negotiate how best to interact could mitigate this.  
%\end{itemize}

And challenges relating to progress in HCI research:
\begin{itemize}
\item 
Blackwell discusses the notion of HCI as an `interdiscipline' \cite{blackwell2015filling,blackwell2015hci} \cite{hornbaek2015we}
\item There have been previous calls for more rigour \cite{whittaker2000let}. What is new this time?

\item Evaluation \cite{heuer2021methods}
\item Research in HCI has, compared with other fields, tended to be a series of `one-shot' prototyping and empirical testing projects, where labs are unable to effectively build on results from other institutions, with little cumulative progress on `motor themes'.\cite{kostakos2015big}. While point studies of usability are of great value in establishing how users understand and use existing interactions, they rarely lead to generalisable models. HCI urgently needs theory-led methods, calibrated with experimental data from users, capable of embedding rich behavioural models in the interaction loop. It also needs us to be able to describe these research findings in objective, consistent and unambiguous fashion to better share the knowledge. \citet{reeves2015human} criticised the focus on the term `science'. \item Reeves suggested that the goals of sciences are Accumulation: Science’s work is that
of cumulative progress,  Replication: Science’s work gains rigor from its replicability,  Generalization: Science’s cumulative work builds toward transcendent
knowledge.
    \item Other fields such as machine learning have made rapid progress on the basis of shared development frameworks and shared code, data and foundation models. Can we reproduce this in HCI? One key issue in interaction design is the sensitivity to the specifics of context (physical environment, culture, social elements). How can we adapt and formalise descriptions of the context in which a model was developed, and its expected domain of validity?
    \item Recent developments in machine learning are providing new technologies which could be valuable for HCI research and practice, but we need to have a principled way of integrating them into the interaction loop.  
\end{itemize}

\subsection{Properties of Computational HCI theories}
Based on the challenges discussed in the previous section, we outline some desirable properties of HCI theory to address the design and analysis of an interactive system. 

\begin{itemize}
    \item {Merits of a Computational approach to interaction.} Constructive, data-driven model-based approaches to human--computer interaction should enable us to make verifiable, measurable progress, and to share that systematically. 
    \item The complexity of the different elements of a human--computer interaction loop means that we will inevitably have a lot of uncertainty in our models, which means that the computational frameworks, software and models need to be probabilistic in nature. \cite{williamson2022introduction,WilOulKri22}.
    \item Modelling will be an ongoing process, with different components and different strata modelled at different levels. Some areas of description will be based on detailed mechanistic models based on robust knowledge in physics, physiology or cognitive science. Others will be black-box models, based largely on data, rather than first principles theory. 
    \item Our models need to be able to incorporate modern technologies such as deep learned neural networks in perception, cognition and action. 
    \item Models will need to be shared with the accompanying data required to calibrate them for specific environments, tasks or users. 

    \item The enhanced role of computational
     models suggests the need for a greater role of simulation \cite{murray2022simulation} in HCI.  The term {\it Simulation Intelligence}, as proposed in \cite{lavin2021simulation} involves the development and integration of the essential algorithms necessary for a merger of scientific computing, scientific simulation, and artificial intelligence. The original paper on this topic focussed on other areas of science and engineering, but the methods are highly relevant to the complex modelling challenges of HCI. 
    \item We need a clear workflow, along the lines proposed by \cite{chandramouli2024workflow}. In general, basing your modelling work around {\it forward} models is more straightforward conceptually and in terms of acquisition of data and application of prior scientific knowledge about the mechanisms involved in the area \cite{MurWilTon22}.
   
     \item Models will need to be generative and predictive.
    \item Closed-loop. Model-based (of the entire closed-loop) analytic measures may be the only realistic way to create measures of concepts such as engagement or agency.

\end{itemize}

\section{Benefits for the research field}
There are potential benefits from this approach for the constructive nature of progress in the field. This has software and engineering aspects, as well as providing analytic benefits.

\citet{van2023implications} proposed seven Implications of HCI research. Can we assess the potential implications of the Active Inference approach?
\begin{itemize}
    \item Implications for methodology. Methodology implications aim to inform the way we design and analyze studies within HCI.
    \item Implications for theory. Theoretical
implications concern the basic
constructs of HCI and our
understanding of how they affect each other.
    \item Implications for the HCI community
    \item Implications for design.
    \item Implications for practice
    \item Implications for policy
    \item Implications for society
\end{itemize}

\subsection{Driving conceptual clarity}

Given its model-based nature, active inference based interaction is likely to face similar criticisms to the general use of modelling and simulation in HCI. These have included: the cost and complexity of developing models, and the inability of models to adequately represent the cognitive and perceptual complexity of the human in the HCI loop, especially given the sensitivity of behavior to details of context. Other critiques have included the perceived failure of models to capture the physical and social context of interaction, leading many researchers and practitioners to argue that traditional human-based usability testing is quicker and more valuable than offline simulation \cite{murray2022simulation}.

Both sides of this argument are typically in agreement that understanding humans is core to successful HCI design. The argument is typically about the level of description involved in the term `understanding humans'. Sheridan emphasises that {\it ``models are the summaries of ideas we hang on to in order to think, communicate to others and refine in order to make progress in the world"} \cite{sheridan2016modeling}, and emphasizes the importance of {\it denotative} model descriptions, which minimize the variability of interpretation, so that the field can agree what it is talking about. {\it ``The process of modelling forces one to think hard about the slice of nature under consideration, to ask and answer the question of what are the essential features of the structure and function, and to make .. predictions"}. So we can argue that the ability to build a generative model that matches user behavior is a strong test of whether we {\it really} understand an interactive system. Furthermore, model-based simulation can support the creation and validation of new theories, and early investment in models can streamline the design and engineering processes, making them more predictable and robust. 

A further aspect of modelling in an active inference context is that the models are constantly coupled to closed-loop control. An ongoing risk in learning models from data is that you can overfit a complex model to a specific dataset or context, but that it does not generalise to a new context, or even to a similar context when you base the control on the model's predictions.

%%%%%%%%%%%%%%%%%%%%%%%
\subsubsection{Components of the new framework}
The standard active inference mechanisms includes the following components. 
\begin{itemize}
    \item {\it System states}, which can include states internal to the agent, states external to the agent, and states which link the agent with the outside world/environment (sensory and action states).
    \item {\it Generative forward models}, which can describe the evolution of the agent's internal states, sensory states, action states and environment states.
    \item {\it Prior distributions}
    \item {\it Inference mechanisms}. Active inference typically uses variational inference for computational efficiency. 
\end{itemize}
 
Active inference depends on minimising the surprise at our sensors. This means that we need a {\it probabilistic generative model} which can predict the expected distribution of sensor observations at any moment. These models are typically flexible models, such as neural networks, which are optimised to be able to act as probabilistic representations of the causes of sensory input and will encode beliefs about observed sensory variables and non-observed hidden variables. 

\subsubsection{Minimising Variational Free Energy}
One technical aspect of active inference is the use of variational approximations of Bayesian inference, to make it computationally tractable. Exact Bayesian inference is computationally intractable because it requires two quantities: the model evidence $P(y)$ and the posterior probability $P(x|y)$. For complex models there may be many types of hidden states which need to be marginalised out, which is computationally intractable. The marginalisation might also require analytically intractable integrals. Variational approaches substitute two intractable quantities (\textit{posterior probability} and \textit{model evidence}) with two quantities that approximate them but which can be computed efficiently, an \textit{approximate posterior} $Q$ and a \textit{variational free energy} $F$.\footnote{In machine learning, the negative variational free energy is known as the evidence lower bound (ELBO).} The Bayesian inference required now becomes an optimisation process.

\subsubsection{Perception as Inference}

In many cases a the generative model will be a simpler approximation of the real-world generative process which causes the sensory observations. Mismatch between the predicted and observed sensory states lead to the agent being `surprised'. 

When we see an unclear object before us we can change our internal beliefs to hypothesise different explanations, or we can adapt our gaze direction or position to get a clearer view of the object, and thus resolve our uncertainty. 

%%%%%%%%%%%%%%%%%%%%%%%%
\section{Removed vignettes}

\subsection{Vignette 1: A number selection system }
\texttt{U () S}

\textbf{Scenario}
\citet{SteWilMur24} implemented active inference in a role interposed between a user and a system requiring numerical entry,  with the caveat that only binary selections can be communicated, and these are heavily corrupted. This is a scenario common in assistive technologies like brain-computer interfaces.  The role of the active inference agent is to facilitate the entry of the intended number reliably (without error) and quickly (with a minimum number of decisions by the user operating it).

\textbf{Actuation and sensing}  Its action space is to choose a "cutpoint" to display to the user, with the  implied question to the user of "is the number you are thinking of above or below this cutpoint?".  Its perception, in this specific task, is a single binary value, 0 or 1, corresponding to the user's response that their intended number is above or below the presented cutpoint. Its perception is clouded by the corruption of the channel so it cannot assume the binary value is a reliable indicator of user intention.

\textbf{Preference prior} What does it prefer? It prefers to be unsurprised by the next binary symbol the user will enter. It also prefers as few symbols as possible to be entered.

\textbf{Forward model} It models the binary digit it next expects to encounter based on a simple model of what an ideal user \textit{would} give were they thinking of a specific number, along with a computational model of the corruption process (e.g. that the channel noise is iid Bernoulli with some bit flip probability).

\textbf{How is surprise minimised?}
To minimise surprise, it must accurately estimate the number the user is thinking of, and disregard deviations induced by the noisy transmission medium. To balance these, such an agent must both act to probe the user (to refine the belief over possible numbers) and probe the channel (to refine the estimate of the channel statistics).

There are several questions resolved simultaneously:
\begin{itemize}
	\item What are the channel properties the user is experiencing? How are inputs being corrupted?
	\item What does the user want to enter? What is the number they are thinking of?
	\item Although not implemented in \cite{SteWilMur24}, it could also reason about how the user has understood the feedback presented to them. What does the user currently believe is going on?
\end{itemize}

\textbf{Why is active inference appropriate?}
 Communicating on the channel is difficult; bits are precious. So the agent must be parsimonious in its calibration effort so as not to over-burden the user. Should it be endowed with a model of how the user is interpreting the feedback presented, it should also reason about how actions which are used to improve estimates of the channel statistics might confuse or interfere with the user's selection process. 

We might also note that had the agent the capacity to compel the user to choose specific targets, it would make its predictions simpler and reduce its surprise. Obviously it is undesirable for the interface to decide what the user wants to do and foist an intention upon the user. But a relaxation of that forced choice would have the agent recommend or support selections it thought were plausible, so as to minimise its own surprise. This assistive support falls naturally out of the active inference principles driving the agent.

\TODO{Should we drop this one as well?}
\begin{revise}
\subsection{Vignette 2: Understanding browsing behaviour }
\texttt{(U) S}
\textbf{Scenario}
How might a \textit{user model} based on active inference be designed? As a concrete example, we imagine modelling how a user browses during a research task like. researching a new model of coffee maker. This user model is intended to produce \textit{in silico} simulations of behaviour, for example to evaluate a sales website before real user trials. There are various theories that can be used to describe how a user might behave, such as information foraging \textbackslash{}cite\{\}. Active inference provides an alternative approach. 

\textbf{Actuation and sensing} 
The simulated user's action space is to scroll up or down; select a hyperlink from the visible page; or to enter a new search term. Their ``sensors'' perceive the text currently visible on the page. While this is the raw sensing that they perceive, we might model the effective sensors as a compressed form of this input, e.g. capturing salient terms from the text presented.

\textbf{Forward model} 
The user's forward model predicts what will be seen if they scroll further through page; what they will see if they click a link; and what results they expect to see if they enter a new search term. 

\textbf{Preference prior}

What does this synthetic user prefer? They prefer to achieve minimal uncertainty over the best coffee makers to choose. To do this, they need to be satisfied they have seen the available universe of coffee makers, and that no additional information remains that will change their ranking of their most valued maker, where value might comprise a combination of pricing, taste satisfaction, volume, percolation time, etc. They also want to spend the minimum time possible researching coffee machines.

\textbf{How is surprised minimised?}

\textbf{Why is active inference appropriate?}

\end{revise}

\subsection{Vignette 5: A business decision support tool }
\TODO{SS to write}

\textbf{Scenario}

\textbf{Actuation and sensing}

\textbf{Forward model} 

\textbf{Preference prior}

\textbf{How is surprised minimised?}

\textbf{Why is active inference appropriate?}

\section{Sharing models}

Similarly, the models will have a strong data-driven element, and we need to improve the quality of our data-management and sharing processes, to allow research groups to manage their own work, and validate the work of other groups.  We anticipate this will create a drive for standardised structures for models of users and of interaction objects, along with procedures for running validation processes, in order to be able to wrap a `validity envelope' around each submodel, which describes the context it was developed in.

%%%%%%%%%%%%%%%%%%%%%%
\item \textbf{Humans are hard to model.}  Humans are individually very complex (cognition, perception and action) and interact socially with other complex humans. This may appear an  insurmountable obstacle for simulation approaches. H Even so, we have relatively few extant computational models and they cover only a limited spectrum of human function.
%\item \textbf{Humans limitations}
%Humans have limited bandwidth in perception, motor control and cognition. These capabilities vary greatly over the population and across situations. While we can perceive very rich states of the world, we only effectively  control a few degrees of  freedom, and are very sensitive to the `handling qualities' of a mechanism. These limits can lead us to design interfaces which are suitably constrained.\footnote{Our devices also have limitations. \citet{janlert2017things} highlight the {\it Interface bottleneck} due to devices with similar complexity getting smaller over time.} This can simplify the inference tasks within coupled active inference agents. However, the bandwidth limitations inherent in our interfaces then force the partners in the dyad into mutual modelling and hence add some more complexity to their mental models \cite{keurulainen2024role}.
\item \textbf{Users  are nonstationary} Humans change  as they learn about their environment, develop skills and learn to use tools, or as their bodies or their preferences evolve. In an active inference-driven interface, the computer's model of the human will have to update throughout this process, and the human's model of the computer will need to update similarly. This leads to to a need to account for recursive theories of mind \cite{keurulainen2024role}. This is computationally and theoretically challenging.
\item \textbf{Environments are increasingly unpredictable} The evolution of mobile, wearable and XR interaction means environments for computing systems have become rapidly more diverse, and thus less knowable. They can change over long or short periods, and can include other sentient, predictive agents. This requires powerful forward models that account for these environments for active inference agents to be resilient.
\item \textbf{Humans are diverse} 
Because of the inevitable variations in the population, we need to be able to cope with diversity in human bodies, behaviour, capabilities, preferences and goals. Engineering adequate diversity in forward models is an open problem.

\item \textbf{Adaptation has risks} Intelligent interfaces have the property that they are less predictable than ``dumb tools''. They adapt and respond in different ways as their internal models improve. Humans, in turn, co-adapt in ways that are not easy to predict. Even if adaptation can theoretically improve interaction, managing user expectations is a challenge.
\item \textbf{Active inference is computationally intensive} 
Inference is computationally complex, particularly in exhaustive action rollouts, and engineering effort will be needed to balance model completeness with the real-time requirements of user interfaces. Amortised algorithms \cite{} will be required to make active inference viable in the interaction loop. Even in offline settings, computational developments will be required to realise the promise of agents with predictive powers on long time horizons.

\item \textbf{Active inference is hard to implement} 
Active inference is an elegant theoretical framework, but we do not yet have the software libraries and computational abstractions to build, reason about, and deploy interfaces. Current implementations of active inference like \texttt{RxInfer}\cite{bagaev2023} and \texttt{pymdp}\cite{heins2022} are nascent and not easily applied for interaction problems. We need tooling akin to the {\it Theano}\footnote{A Python library to define, optimize, and efficiently evaluate expressions involving multi-dimensional arrays, which kickstarted the standardisation and sharing of deep-learning architectures. Tensorflow, PyTorch and JAX are descendents of Theano.} of modern interaction design. We also lack developed workflows \cite{gelman2020bayesian,chandramouli2024workflow} to support the application of active inference to interaction. We need new, principled, computational human-centric engineering design to capture human behaviour and acquire the data necessary to build preference priors and forward models.
\item \textbf{Preference priors require thought} Active inference eschews rewards for the flexibility of preference priors. Casting interaction problems in terms of these novel approaches to preference is flexible but unfamiliar. How should preference priors be elicited? How should they be validated? How can generalised preferences be fused from individual elicitations? These are open questions. 

\item \textbf{Uncertainty and prediction are unfamiliar} Representing uncertainty can make interfaces robust but users can struggle to comprehend uncertainty (Section \ref{sec:uncertainty}). Prediction is a vital component of active inference and can mitigate latency and delays in the interaction loop. But prediction can be unsettling for users. This predictive, pro-active nature, may initially make interfaces endowed with AIF models appear to be in the `uncanny valley' \cite{mori1970bukimi}.
 Managing this is important if predictive agents are to form part of interactive systems.

 %%%%%%%%%%%%%%%%%%%
 \subsubsection{What can Markov Blankets do for HCI?}
Markov blankets have clear value as sharp intellectual tools for segmenting functional roles in interactive systems. Markov blankets could be \textbf{detected}; we can use formal statistical measures to identify  blankets from data, informing us how the boundary between human and computer shifts. In fact, we should see the re-forming of the Markov blanket over time as the means by which long term surprisal is minimized. If an agent cannot preserve a Markov blanket, it has no internal states, and hence dissolves into its environment. In his attempt to compare the nature of human and machine intelligence, \citet{lawrence2024atomic} looks at what the `atomic' core of humanity is, the elements which cannot be replaced by AI. Markov blankets offer an instrument to quantify what happens to users of sensory and cognitive augmentative technology as their boundaries shift over time. We can also \textbf{define} Markov blankets to support interaction. However, it is not yet clear how best to represent this in interaction engineering, and to what degree it can be used to constrain adaptation or help support calibration.
